# Supplementary material for: A sufficient set of experimentally implementable thermal operations
Source: arXiv:1511.06553 source file (2016-10-10)
Supplement: Supplementary file 3 [file definitions.tex]

\def\<{\langle}
\def\>{\rangle}

\newcommand{\be}{\begin{eqnarray} \begin{aligned}}
\newcommand{\ee}{\end{aligned} \end{eqnarray} }
\newcommand{\benn}{\begin{eqnarray*} \begin{aligned}}
\newcommand{\eenn}{\end{aligned} \end{eqnarray*} }

\newcommand{\ben}{\begin{eqnarray} \begin{aligned}}
\newcommand{\een}{\end{aligned} \end{eqnarray} }

\newcommand{\bc}{\begin{center}}
\newcommand{\ec}{\end{center}}

				% VECTORS
				% ABS

%
%\newtheorem{theorem}{Theorem}[section]
%\newtheorem{proposition}{Proposition}[section]
%MH
\newcommand{\beq}{\begin{eqnarray} \begin{aligned}}
\newcommand{\eeq}{\end{aligned} \end{eqnarray} }
\newcommand{\bea}{\begin{array}}
\newcommand{\eea}{\end{array}}

\newcommand{\bee}{\begin{enumerate}}
\newcommand{\eee}{\end{enumerate}}
\newcommand{\bei}{\begin{itemize}}
\newcommand{\eei}{\end{itemize}}

%MH

  %%% Space spanned by a set of vectors.

%\newcommand{\note}[1]{\textsc{#1} $\clubsuit$}

%%%%%%%%%%%%%% Greek Letters %%%%%%%%%%%%%%%%%%%%%%

\usepackage{amsfonts}

\def\01{\{0,1\}}

 % inproduct, < | >

%\newcommand{\eeq}{\end{align}}
%\newcommand{\beq}{\begin{align}}

%\newcommand{\supl}{Supplementary Materials}

\def\<{\langle}
\def\>{\rangle}

%_\alpha(#1,H)}
% oh no, I can't believe we're hatting, especially here!

%_\alpha(#1,H)}
%Michal's defs

% jono'ss

%\newtheorem*{rep@theorem}{\rep@title}
\newcommand{\newreptheorem}[2]{%
\newenvironment{rep#1}[1]{%
 \def\rep@title{#2 \ref{##1} (restatement)}%
 \begin{rep@theorem}}%
 {\end{rep@theorem}}}
\makeatother

\newreptheorem{thm}{Theorem}
\newreptheorem{lem}{Lemma}
