# Supplementary material for: A sufficient set of experimentally implementable thermal operations
Source: arXiv:1511.06553 source file (2016-10-10)

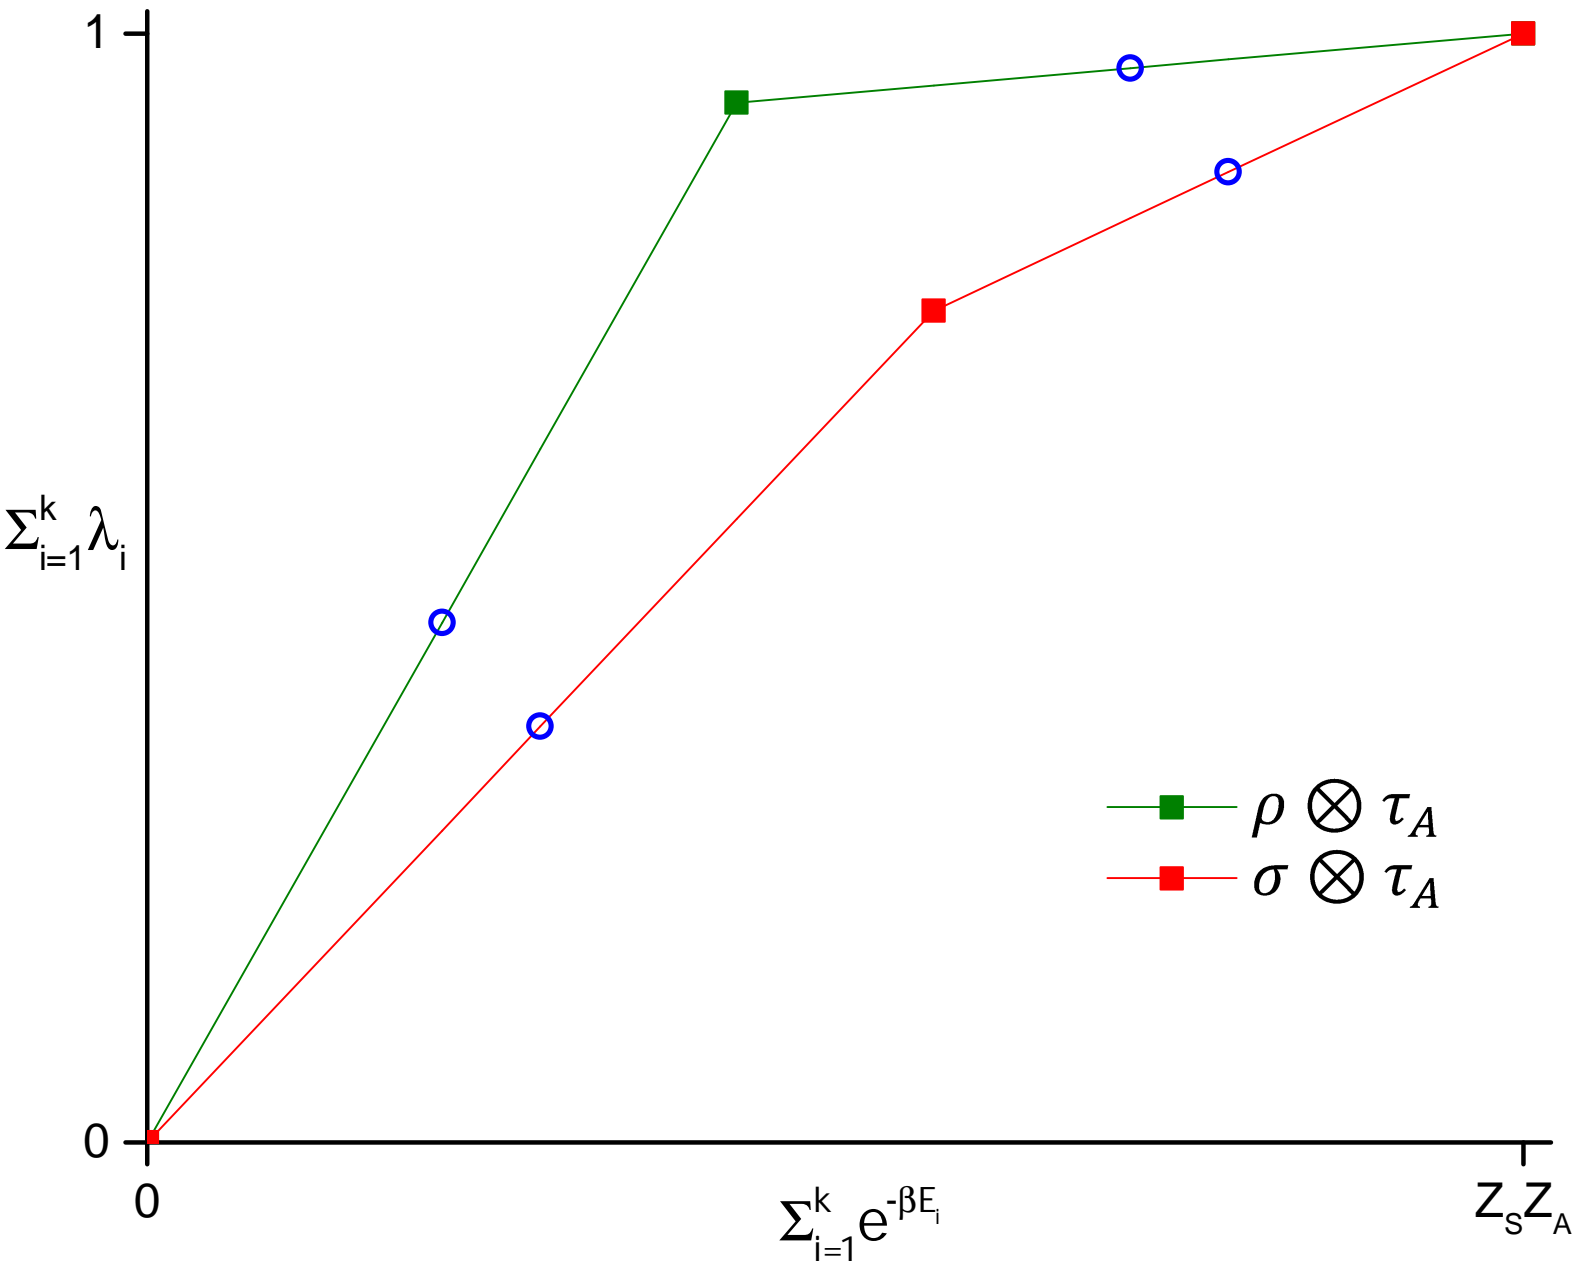

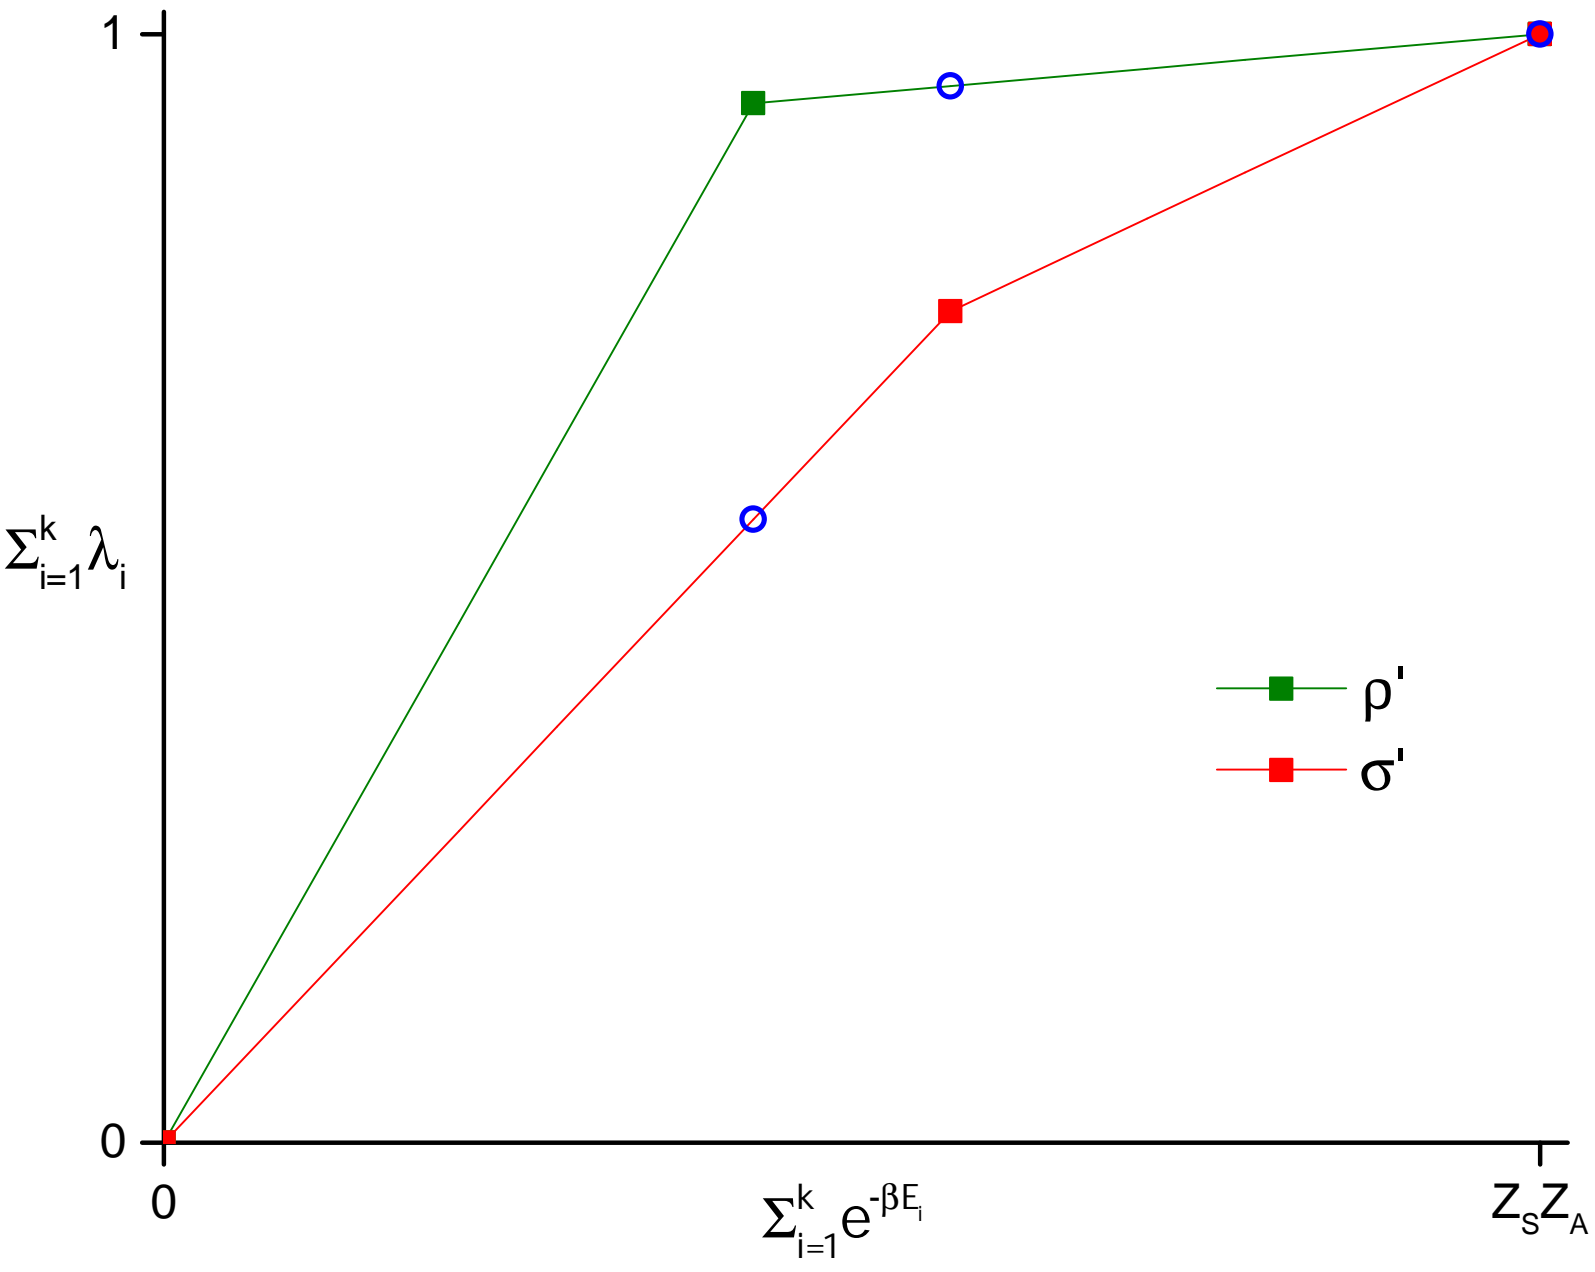

Supplement: Supplementary file 4 [file Sketch_-_Beta_order_change__with_infinity_.pdf]
